# Supplementary material for: Redox-controlled epitaxy and magnetism of oxide heterointerfaces: EuO/SrTiO$_3$
Source: arXiv:1902.06301 ancillary file (2019-02-17)
Supplement: Supplementary file 1 [file supplementary_materials.pdf]

# Supplementary Materials: Redox-controlled epitaxy and magnetism of oxide heterointerfaces: $EuO/SrTiO_3$

Patrick Lömker[1,2] and Martina Müller[2,3,*]

[1]Photon Science, Deutsches Elektronen Synchrotron, D-22607 Hamburg, Germany
[2]Peter Grünberg Institut (PGI-6), Forschungszentrum Jülich GmbH, D-52428 Jülich, Germany
[3]Fakultät Physik, Technische Universität Dortmund, D-44221 Dortmund, Germany

(Dated: February 17, 2019)

We present the structural changes of Eu metal as it is oxidized into EuO, an Ellingham analysis for the most stable oxide of Eu at the $SrTiO_3$ surface and the methodology for the determination of thicknesses applied in the results and outlook part of the main manuscript.

## I. SUBSTRATE PREPARATION AND EU DEPOSITION

Single crystalline 5 mm × 5 mm Nb:$SrTiO_3$ (001) (Crystec) were used as substrates in this study. The substrates are $TiO_2$-terminated using buffered hydrofluoric acid etching and annealing by established procedure [1]. The prepared surfaces are flat with steps of unit cell height and a small roughness within a terrace is observed with atomic force microscopy ($R_a$ <150 pm). The miscut angle is in the interval 0.05 to 0.10 deg resulting in a terrace width of 200 to 500 nm. The substrates are n-doped with 0.5 wt% Nb to avoid charging during electron diffraction and spectroscopy.

A molecular beam epitaxy (MBE) system with base pressure $p < 3 \times 10^{-10}$ mbar is used for the *in situ* preparation (SPECS). Prior to Eu deposition, the substrates were subjected to an annealing step at 600 °C for 0.5 h using a local oxygen partial pressure of $1 \times 10^{-7}$ Torr (purity 99.996% $O_2$). This provides chemically clean and structurally sharp surfaces. Pure Eu metal (purity 99.97 %) is evaporated at 580 °C from a low temperature Knudsen cell, at a rate of $j_{\mathrm{Eu}} = 0.13\,\text{Å}\,\mathrm{s}^{-1}$. The rate is measured with a calibrated quartz micro balance. We determine the substrate temperature, using a single wave length pyrometer set to the emissivity of $\epsilon = 0.35$ and report the direct pyrometer read outs as $T_P$ [2].

## II. *EX SITU* CHARACTERIZATION

Prior to *ex situ* characterization all samples are capped by 10 nm MgO, in order to avoid further (over)-oxidation. A reciprocal space map and X-ray reflectometry are recorded using the Cu $K_\alpha$ line in a four circle diffractometer (Philips). Magnetization measurements are conducted using a SQUID magnetometer and a vibrating sample magnetometer (Quantum Design). Hysteresis loops of $H = \pm 1500$ Oe are performed at $T = 5$ K and the temperature dependence is recorded with an aligning field of $H = 500$ Oe for $T =$ 5 to 150 K. All magnetization data was measured in-plane.

* mart.mueller@fz-juelich.de

## III. PREPARATION OF EU REFERENCE SPECTRA

We use yttria-stabilized zirconia (YSZ) as a substrate to prepare $d = 10$ nm thick films of Eu metal at room temperature with no added oxygen, EuO at $T = 500$ °C with a 1:1 ratio between adsorbed Eu and O and $Eu_3O_4$ supplying three times as much O as Eu at $T = 500$ °C. In this we use the established adsorpiton limited preparation method for this substrate [3]. At room temperature we measure XPS of the Eu $3d_{5/2}$ core-level and present the normalized data in Fig. 1(a). The shape for the pure $Eu^{3+}$ valence that is found in $Eu_2O_3$ is obtained by subtracting the data for pure EuO from the data obtained from the $Eu_3O_4$ film.

## IV. CRYSTAL STRUCTURE OF EU AND EUO

The redox process we describe in our manuscript between the metallic reactant Eu and the oxide $SrTiO_3$ leads to a structural modification of the growing Eu overlayer: The impinging Eu metal crystallizes in a body centered (bcc) crystal structure with $V_{Eu} = 96.07\,\text{Å}^3$/u.c. with 2 Eu atoms per unit cell [4, 43578]. However, upon oxidation, stoichiometric EuO takes a rock-salt (NaCl) crystal structure with $a_{EuO} = 135.96\,\text{Å}^3$/u.c. [4, 53437] with 4 Eu atoms per unit cell. This accounts for a volume shrinking (per Eu atom) to 71.1 %. Therefore, the redox-growth of 1 ML = 2.57 Å of EuO requires the evaporation of 3.61 Å of Eu metal. Also the well known temperature dependent re-evaporation of Eu metal from the surface causes the reading of the quartz micro balance to be an upper boundary to the real film thickness only.

## V. ELLINGHAM ANALYSIS

The thermodynamic potentials govern the equilibrium state of the prepared films. As a measure for the direction of a reaction an Ellingham analysis can be conducted [5]. The change of the Gibbs free energy ($\Delta_r G^0$) needs to be calculated as a function of temperature for the probable oxidation reactions of the metallic elements involved. The

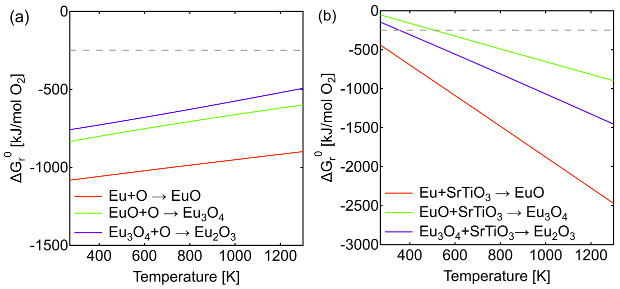


Figure 1. Ellingham diagram of (a) europium oxides in the adsorption limited case and (b) europium oxides formed by reduction of a $SrTiO_3$ substrate .

values for the Gibbs free energy are obtained from standard tabulated values for Eu-, Sr-, Ti- and their oxides, and $SrTiO_3$ are calculated for higher temperatures on the basis of tabulated values found in the literature [6–9].

The involved elemental reactions are

$$2\,Eu + O_2 \rightleftarrows EuO \quad (1)$$
$$6\,EuO + O_2 \rightleftarrows 2\,Eu_3O_4 \quad (2)$$
$$4\,Eu_3O_4 + O_2 \rightleftarrows 6\,Eu_2O_3 \quad (3)$$
$$4\,SrO + 2\,Ti_2O_3 + O_2 \rightleftarrows 4\,SrTiO_3 \quad (4)$$

The possible chemical reactions taking place at the $EuO/SrTiO_3$ interface are

$$2\,Eu + 4\,SrTiO_3 \rightarrow 2\,EuO + 4\,SrO + 2\,Ti_2O_3 \quad (5)$$
$$6\,EuO + 4\,SrTiO_3 \rightarrow 2\,Eu_3O_4 + 4\,SrO + 2\,Ti_2O_3 \quad (6)$$
$$4\,Eu_3O_4 + 4\,SrTiO_3 \rightarrow 6\,Eu_2O_3 + 4\,SrO + 2\,Ti_2O_3 \quad (7)$$

All these reactions are thermodynamically feasible (i.e. they over-come the minimal Gibbs free energy of formation $\Delta_r G^0 > 250\,\mathrm{kJ\,mol^{-1}}$ ) for temperatures above $T_S \geq 400\,°C$. Therefore an oxidation to the highes oxide is a possible result of reducing the $SrTiO_3$ surface and $Eu_2O_3$ is therefore the equilibirum oxide.

Fig. 1 shows the behavior of Europium and its oxides in general (part (a)) and in proximity to $SrTiO_3$ (part (b)) by the aforementioned reactions. We can deduce that $SrTiO_3$ is a suitable candidate for redox EuO growth on $SrTiO_3$, as the oxidation of Eu metal is favored when compared to the reduction of Eu oxides on $SrTiO_3$.

## VI. THICKNESS DETERMINATION WITH X-RAYS

For the thickness dependence in the results chapter we use the Beer-Lambert law on the buried $TiO_2$ layers of the $SrTiO_3$ crystal. The intensity of the Ti $2p$ core-level $I_B$ is then given by

$$I_B = I_0 \exp(-d/\lambda_{substrate}) \quad (8)$$

where the inelastic mean free path of the photoelectrons from the Ti $2p$ in the Eu-film is taken from literature $\lambda_{substrate} = 1.89\,\mathrm{nm}$, $I_0$ is the intensity of the bare substrate and $d$ denotes the thickness of the grown overlayer [10] .

For the films in the outlook, shown in Fig. 6(a) we use the intensity of the Eu-film as a gauge for the thickness, as the substrates may be highly insulating and charging effects made a study of the substrate impossible. As all films are of comparable thickness to the inelastic mean free path of the photoelectrons excited by the Al $K_\alpha$ X-rays, it is possible to obtain the film thickness from the total intensity $I(d)$ of the Eu $3d_{5/2}$ peak

$$I(d) = I_\infty(1 - \exp(-d/\lambda_{film})), \quad (9)$$

where $I_\infty$ is the intensity of an infinitely thick film, $d$ is the film thickness and $\lambda_{film}$ is the inelastic mean free path of photoelectrons from the Eu $3d_{5/2}$ core-level in the Eu-oxide. It is taken from the literature for Gd as an estimate to be $\lambda_{film} = 0.776\,\mathrm{nm}$ [10].

[1] G. Koster, B. L. Kropman, G. J. H. M. Rijnders, D. H. A. Blank, and H. Rogalla, Quasi-ideal strontium titanate crystal surfaces through formation of strontium hydroxide, Appl. Phys. Lett. **73**, 2920 (1998).
[2] Prinsen, *Nucleation and Growth on SrTiO 3 Substrates Characterize by Ex-Situ AFM*, Ph.D. thesis (2007).
[3] R. Sutarto, S. G. Altendorf, B. Coloru, M. Moretti Sala, T. Haupricht, C. F. Chang, Z. Hu, C. Schüßler-Langeheine, N. Hollmann, H. Kierspel, H. H. Hsieh, H.-J. Lin, C. T. Chen, and L. H. Tjeng, Epitaxial and layer-by-layer growth of EuO thin films on yttria-stabilized cubic zirconia (001) using MBE distillation, Phys. Rev. B **79**, 205318 (2009).
[4] G. Bergerhoff and I. D. Brown, Inorganic Crystal Structure Database, in *Crystallographic Databases*, edited by F. H. Allen, G. Bergerhoff, and R. Sievers (International Union of Crystallography, Bonn/Cambridge/Chester, 2017) pp. 77–95.
[5] H. J. T. Ellingham, Reducibility of Oxides and Sulphides in Metallurgical Processes, J Soc Chem Ind **63**, 125 (1944).
[6] R. J. Konings, O. Beneš, A. Kovács, D. Manara, D. Sedmidubský, L. Gorokhov, V. S. Iorish, V. Yungman, E. Shenyavskaya, and E. Osina, The Thermodynamic Properties of the f-Elements and Their Compounds. Part 2. The Lanthanide and Actinide Oxides, J Phys Chem Ref Data **43**, 013101 (2014).
[7] Collaboration: Scientific Group Thermodata Europe (SGTE), Thermodynamic Properties of Compounds, SbO to SO2, in *Pure Substances. Part 4 Compounds from HgHg to ZnTeg*, Vol. 19A4, edited by Lehrstuhl für Theoretische Hüttenkunde and Rheinisch-Westfälische Technische Hochschule Aachen (Springer-Verlag, Berlin/Heidelberg,

2001) pp. 275–300.

[8] Collaboration: Scientific Group Thermodata Europe (SGTE), Thermodynamic Properties of Compounds, SbO2 to Rh2O3, in *Pure Substances. Part 4 Compounds from HgHg to ZnTeg*, Vol. 19A4, edited by Lehrstuhl für Theoretische Hüttenkunde and Rheinisch-Westfälische Technische Hochschule Aachen (Springer-Verlag, Berlin/Heidelberg, 2001) pp. 301–324.

[9] M. Adachi, Y. Akishige, T. Asahi, K. Deguchi, K. Gesi, K. Hasebe, T. Hikita, T. Ikeda, Y. Iwata, M. Komukae, T. Mitsui, E. Nakamura, N. Nakatani, M. Okuyama, T. Osaka, A. Sakai, E. Sawaguchi, Y. Shiozaki, T. Takenaka, K. Toyoda, T. Tsukamoto, and T. Yagi, SrTiO3 Survey, 1A-8, in *Oxides*, Vol. 36A1, edited by Y. Shiozaki, E. Nakamura, and T. Mitsui (Springer-Verlag, Berlin/Heidelberg, 2002) pp. 1–7.

[10] S. Tanuma, C. J. Powell, and D. R. Penn, Calculations of electron inelastic mean free paths. IX. Data for 41 elemental solids over the 50 eV to 30 keV range, Surf. Interface Anal. **43**, 689 (2011).
